# Supplementary material for: Beyond Image Super-Resolution for Image Recognition with Task-Driven Perceptual Loss
Source: arXiv:2404.01692 source file (2024-04-04)
Supplement: Supplementary file 1 [file baseline_corrected.tex]

% \begin{table}
% \small
% \centering
% \setlength\tabcolsep{1.0pt}
% \def\arraystretch{1.1}
% \begin{tabular}{C{2.5cm}|C{1.3cm}|C{1.3cm}|C{2.0cm}}
% \specialrule{.1em}{.05em}{.05em}
% \hline
% Methods & PSNR & SSIM & MACs \\
% \specialrule{.1em}{.05em}{.05em}
% Baseline & 30.43 & 0.9050 & 13.79 \\
% % Baseline$^\text{chan+}$ & 30.46 & 0.9053 & 14.64 \\
% % \hline
% ClassConv & 30.67 & 0.9085 & (0.52) + 13.79 \\
% \hline
% \specialrule{.1em}{.05em}{.05em}
% \end{tabular}
% \caption{
%     \textbf{Performance of the proposed ClassConv.} 
%     sample.
% }
% \label{table:baseline}
% \end{table}

\begin{table}
\small
\centering
\setlength\tabcolsep{1.0pt}

\begin{tabular}{L{2.2cm}C{1.1cm}C{1.1cm}C{1.6cm}C{1.6cm}}
\toprule
\,~\multirow{2}{*}{Methods} & \multicolumn{2}{c}{GoPro} & \multirow{2}{*}{MACs~(G)} & \multirow{2}{*}{Latency~(s)} \\
& PSNR & SSIM & &\\
\hline
% \;~U-Net & 30.43 & 0.9049 & 13.79 & 2.61 \\
% \;~+~\textbf{B-conv} & 30.67 & 0.9081 & +~0.52 & +~4.30 \\
% % Conv (+chan) & 30.46 & 0.9053 & 14.64 & & 2.78 \\
% \hline
% \;~Baseline~\cite{db_nafnet} & 32.24 & 0.9311 & 15.96 & 17.0\\
% \;~+~\textbf{B-conv} & 32.34 & 0.9321 & +~0.52 & +25.9\\
% \hline
% \;~NAFNet~\cite{db_nafnet} & 32.31 & 0.9321 & 12.29 & 12.1\\
% \;~+~\textbf{B-conv} & 32.36 & 0.9326 & +~0.52 & + 17.6\\

\;~U-Net & 30.43 & 0.9049 & 13.79 & 0.265 \\
\;~+~\textbf{B-conv} & 30.67 & 0.9081 & 14.31 & 0.333 \\
% Conv (+chan) & 30.46 & 0.9053 & 14.64 & & 2.78 \\
\hline
\;~Baseline~\citenumber{2} & 32.24 & 0.9311 & 15.96 & 0.284 \\
\;~+~\textbf{B-conv} & 32.34 & 0.9321 & \textcolor{BrickRed}{16.48} & 0.362 \\
\hline
\;~NAFNet~\citenumber{2} & 32.31 & 0.9321 & 12.29 & 0.231 \\
\;~+~\textbf{B-conv} & 32.36 & 0.9326 & \textcolor{BrickRed}{12.81} & 0.287 \\

\bottomrule
\end{tabular}
\caption{
    \textbf{Advantage of applying B-conv to various deblurring architectures.}
    We denote the corrected value as \textcolor{BrickRed}{\textbf{red}} color.
}
\label{table:baseline_performance_corrected}
\end{table}
